# Supplementary material for: OAMixer: Object-aware Mixing Layer for Vision Transformers
Source: arXiv:2212.06595 source file (2022-12-13)
Supplement: Supplementary file 1 [file additional.tex]

\section{Additional results and comparisons with prior methods}
\label{appx:additional}

We provide additional results on various scenarios, e.g., comparison with prior methods. To this end, we conduct experiments on the Background Challenge \cite{xiao2020noise} benchmark, which consists of a smaller (9 superclass, 370 class) subset of ImageNet as a training dataset, called ImageNet-9 (IN-9), and eight test datasets to evaluate the classification and background robustness.\footnote{
We also provide the results using a larger version of IN-9 (IN-9L) as a training dataset in Appendix~\ref{appx:in9l}. It improves the overall performance of all models but shows a similar tendency with IN-9.
} In this section, we will demonstrate that (a) ReMixer improves background robustness, ReMixer outperforms (b) prior methods using spatial inductive bias and (c) prior methods using patch-level supervision, (d) ReMixer also works well for other patch-based models, and (e) ReMixer can be generalized on distribution shifts. In addition, we compare ReMixer using different object labels in Appendix~\ref{appx:bigbigan}.

\textbf{Setup.}
Background Challenge contains eight evaluation datasets with different combinations of foregrounds and backgrounds: \textsc{Original}~($\uparrow$), \textsc{Only-BG-B}~($\downarrow$), \textsc{Only-BG-T}~($\downarrow$), \textsc{No-FG}~($\downarrow$), \textsc{Only-FG}~($\uparrow$),  \textsc{Mixed-Same}~($\uparrow$), \textsc{Mixed-Rand}~($\uparrow$), \textsc{Mixed-Next}~($\uparrow$), where the upper or lower arrows imply the model should predict the class well or not, respectively. Namely, the model should increase the accuracy of ($\uparrow$) datasets while decrease the accuracy (or increase the background robustness) of ($\downarrow$) datasets. We also report \textsc{BG-Gap}~($\downarrow$) which measures the accuracy gap between \textsc{Mixed-Same} and \textsc{Mixed-Rand}. We omit \textsc{Only-BG-T}, \textsc{No-FG}, \textsc{Only-FG}, and \textsc{Mixed-Next} results for the brevity (see Appendix~\ref{appx:bg_challenge} for discussion). We use ReLabel trained on ImageNet for all following experiments, but ReLabel trained on IN-9 gives similar trends (see Appendix~\ref{appx:relabel_in9}).

\textbf{Background robustness.}
Table~\ref{tab:bg} presents the results on the Background Challenge benchmark, which has several additional implications that will be discussed in a few following paragraphs. First, we remark that ReMixer consistently improves the classification and background robustness in all considered scenarios. To highlight a few numbers, ReMixer enhances the classification accuracy of DeiT-T from 70.62\% to 81.98\% (+11.36\%) on the \textsc{Original} dataset while reducing the background bias of DeiT-S from  39.46\% to 31.78\% (-7.68\%) on the \textsc{Only-BG-B} dataset. These results support that ReMixer learns more object-centric representation robust to background shifts.

\textbf{Comparison with methods using spatial inductive bias.}
We compare ReMixer with patch mixing layers using spatial inductive bias: ConViT \cite{d2021convit} and CoAtNet \cite{dai2021coatnet}. We only take the modified patch mixing layers from both models and apply them to DeiT for a fair comparison. Both ConViT and CoAtNet calibrate self-attention but use spatial distance instead of semantic distance from object labels. We keep the last two layers of ConViT as the vanilla self-attention following the original paper. Table~\ref{tab:bg} shows that ReMixer outperforms both ConViT and CoAtNet for all considered scenarios. Notably, the DeiT-T results show that spatial inductive bias often not help background robustness, as local aggregation does not prevent the entangling of patches in adjacent regions. We also remark that combining ConViT and ReMixer performs the best; they give orthogonal benefits.

\textbf{Comparison with methods using patch-level supervision.}
We compare ReMixer with prior work using patch-level supervision, TokenLabeling (TL) \cite{jiang2021all}. Specifically, TL uses the object (or patch) labels as an additional objective for each patch. We remark that TL and ReMixer benefit the model differently, and using both performs the best. Table~\ref{tab:bg} shows that ReMixer+TL outperforms TL for all considered scenarios. It confirms that the advantage of ReMixer comes from the guided patch interaction, not only from the usage of patch-level supervision. In particular, we highlight that TL does not improve the background robustness, unlike ReMixer gives a significant gain.

\textbf{ReMixer on various patch-based models.}
We apply ReMixer to MLP-Mixer \cite{tolstikhin2021mlp} and ConvMixer \cite{trockman2022patches}, representative patch-based models using feed-forward and convolutional patch mixing layers. We adopt the architecture of ConvMixer to follow the configuration of MLP-Mixer-S/16 (dim: 512, depth: 8) for a fair comparison among Mixers (denoted as ConvMixer-S/16) and use a kernel size of 9 for convolution following the original setup. We share the convolution kernel over channels (see Appendix~\ref{appx:convmixer} for the unshared results). We follow the same training scheme of DeiT for all models. Table~\ref{tab:bg} shows that ReMixer also works well for other patch-based models.

\textbf{Generalization on distribution shifts.}
Table~\ref{tab:dist-shift} shows the classification accuracy of models trained on ImageNet-9, evaluated on various distribution-shifted datasets: 9 superclass (370 class) subsets of ImageNetV2~\cite{recht2019imagenet}, ImageNet-ReaL~\cite{beyer2020we}, ImageNet-Rendition~\cite{hendrycks2021many}, ImageNet-Stylized~\cite{geirhos2018imagenet}, and ImageNet-Sketch~\cite{wang2019learning}, denoted by adding `-9' at the suffix of their names. ReMixer also generalizes well on distribution shifts. We use BigBiGAN for object labels since it worked better than ReLabel; finding salient regions is easier than predicting semantics for the unseen samples.

\begin{table*}[t]
\caption{
Comparison of various scenarios evaluated on the Background Challenge benchmark. We report the classification accuracy (\buparrow) and background robustness (\rdownarrow), where higher and lower values are better for each metric. ``TL'' (gray lines) indicates TokenLabeling, that the model is trained with an additional token-level objective. We use ReLabel from ImageNet trained model for both ReMixer and TL. `+' denotes the modules added to the baseline (not accumulated), and parenthesis denotes the gap from the baseline. The table has several implications: (a) ReMixer consistently improves the classification and background robustness, confirming the benefit of object-centric representation. (b) ReMixer outperforms the methods using spatial inductive bias like ConViT and CoAtNet; combining with ReMixer performs even better. (c) ReMixer gives additional gain over TL, verifying the merit of guided patch interaction over na\"ive patch-level objective. (d) ReMixer also improves MLP-Mixer and ConvMixer, patch-based models using different patch mixing layers.
}\label{tab:bg}
\vspace{-0.1in}
\centering\small
\begin{tabular}{lclllll}
\toprule
& TL & Original (\buparrow) & Only-BG-B (\rdownarrow) & Mixed-Same (\buparrow) & Mixed-Rand (\buparrow) & BG-Gap (\rdownarrow)\\
\midrule
DeiT-T           & - & 70.62 & 35.48 & 63.31 & 39.56 & 23.75 \\
+ ConViT         & - & 78.74 \bup{8.12} & 38.69 \bup{3.21} & 70.84 \bup{7.53} & 46.91 \bup{7.35} & 23.93 \bup{0.18}  \\
+ CoAtNet        & - & 78.62 \bup{8.00} & 37.68 \bup{2.20} & 70.40 \bup{7.09} & 45.46 \bup{5.90} & 24.94 \bup{1.19}  \\
+ ReMixer (ours) & - & 81.98 \bup{11.36} & 30.89 \rdown{4.59} & 73.38 \bup{10.07} & 51.53 \bup{11.97} & 21.85 \rdown{1.90}  \\
+ ReMixer + ConViT (ours) & - & 83.38 \bup{12.76} & 31.36 \rdown{4.12} & 74.86 \bup{11.55} & 53.14 \bup{13.58} & 21.73 \rdown{2.02}  \\
\rowcolor{lightgray}
DeiT-T           & \checkmark & 83.50 & 37.01 & 74.57 & 51.78 & 22.79 \\
\rowcolor{lightgray}
+ ReMixer (ours) & \checkmark & 87.23 \bup{3.73} & 29.21 \rdown{7.80} & 78.15 \bup{3.58} & 60.59 \bup{8.81} & 17.56 \rdown{5.23} \\
\midrule
DeiT-S           & - & 82.69 & 39.46 & 73.88 & 50.49 & 23.39\\
+ ConViT         & - & 85.51 \bup{2.82} & 38.94 \rdown{0.52} & 76.40 \bup{2.52} & 54.37 \bup{3.88} & 22.03 \rdown{1.36}  \\
+ ReMixer (ours) & - & 86.32 \bup{3.63} & 31.78 \rdown{7.68} & 78.44 \bup{4.56} & 56.74 \bup{6.25} & 21.70 \rdown{1.69}  \\
+ ReMixer + ConViT (ours) & - & 88.20 \bup{5.51} & 30.79 \rdown{8.67} & 79.16 \bup{5.28} & 60.52 \bup{10.03} & 18.64 \rdown{4.75}  \\
\rowcolor{lightgray}
DeiT-S           & \checkmark & 88.52 & 38.00 & 79.43 & 59.36 & 20.07 \\
\rowcolor{lightgray}
+ ReMixer (ours) & \checkmark & 91.31 \bup{2.79} & 29.19 \rdown{8.81} & 81.78 \bup{2.35} & 66.92 \bup{7.56} & 14.86 \rdown{5.21} \\
\midrule
MLP-Mixer-S/16   & - & 84.99 & 40.96 & 76.52 & 54.72 & 21.80\\
+ ReMixer (ours) & - & 87.68 \bup{2.69} & 27.28 \rdown{13.68} & 79.43 \bup{2.91} & 60.44 \bup{5.72} & 18.99 \rdown{2.81}  \\
\rowcolor{lightgray}
MLP-Mixer-S/16   & \checkmark & 88.07 & 38.17 & 79.21 & 58.72 & 20.49 \\
\rowcolor{lightgray}
+ ReMixer (ours) & \checkmark & 90.49 \bup{2.42} & 28.72 \rdown{9.45} & 81.63 \bup{2.42} & 65.36 \bup{6.64} & 16.27 \rdown{4.22} \\
\midrule
ConvMixer-S/16   & - & 86.32 & 41.38 & 78.59 & 56.99 & 21.60\\
+ ReMixer (ours) & - & 88.49 \bup{2.17} & 35.60 \rdown{5.78} & 81.70 \bup{3.11} & 63.93 \bup{6.94} & 17.77 \rdown{3.83}  \\
\rowcolor{lightgray}
ConvMixer-S/16   & \checkmark & 87.49 & 36.49 & 80.42 & 58.15 & 22.27 \\
\rowcolor{lightgray}
+ ReMixer (ours) & \checkmark & 89.09 \bup{1.60} & 32.67 \rdown{3.82} & 82.64 \bup{2.22} & 63.70 \bup{5.55} & 18.94 \rdown{3.33}\\
\bottomrule
\end{tabular}
\end{table*}

\begin{table*}[t]
\caption{
Classification accuracy on various distribution-shifted datasets. Bold denotes the best results, and parenthesis denotes the gap from the baseline. ReMixer gives consistent improvements.
}\label{tab:dist-shift}
\vspace{-0.1in}
\centering\small
% \resizebox{0.95\textwidth}{!}{% 
\begin{tabular}{ll|lllll}
\toprule
& ImageNet-9 & ImageNetV2-9 & ReaL-9 & Rendition-9 & Stylized-9 & Sketch-9 \\
\midrule
DeiT-T           & 70.62 & 63.19 & 68.13 & 24.14 & 16.66 & 21.65 \\
+ ReMixer (ours) & \textbf{80.15} \up{9.53} & \textbf{70.68} \up{7.49} & \textbf{77.78} \up{9.65} & \textbf{27.53} \up{3.39} & \textbf{21.80} \up{5.14} & \textbf{24.45} \up{2.80} \\
\midrule
DeiT-S           & 82.69 & 73.22 & 80.21 & 28.60 & 21.90 & 27.26 \\
+ ReMixer (ours) & \textbf{83.88} \up{1.19} & \textbf{75.68} \up{2.46} & \textbf{82.37} \up{2.16} & \textbf{29.43} \up{0.83} & \textbf{24.64} \up{2.74} & \textbf{27.93} \up{0.67} \\
\midrule
MLP-Mixer-S/16   & 84.99 & \textbf{76.57} & 82.70 & 34.25 & 25.54 & 37.07 \\
+ ReMixer (ours) & \textbf{86.30} \up{1.31} & 76.51 \down{0.06} & \textbf{83.37} \up{0.67} & \textbf{34.29} \up{0.04} & \textbf{27.08} \up{1.54} & \textbf{38.16} \up{1.09} \\
\midrule
ConvMixer-S/16   & 86.32 & 76.38 & 83.16 & 33.33 & 24.21 & 34.36 \\
+ ReMixer (ours) & \textbf{86.35} \up{0.03} & \textbf{76.97} \up{0.59} & \textbf{83.56} \up{0.40} & \textbf{33.81} \up{0.48} & \textbf{24.94} \up{0.73} & \textbf{35.72} \up{1.36} \\
\bottomrule
\end{tabular}
\end{table*}
