# Supplementary material for: OAMixer: Object-aware Mixing Layer for Vision Transformers
Source: arXiv:2212.06595 source file (2022-12-13)
Supplement: Supplementary file 6 [file exp_setup.tex]

\section{Experimental setup}
\label{appx:exp-setup}

\textbf{Models and training.}
We mainly apply ReMixer on the DeiT \cite{touvron2021training} and MobileViT \cite{mehta2022mobilevit} architectures, representative patch-based models using a self-attention patch mixing layer. We follow the default training setup of DeiT: train the models for 300 epochs using the suggested augmentation scheme, but with a reduced batch size of 256. Our code is implemented on top of the official DeiT code and PyTorch Image Models (timm) \cite{rw2019timm} library.

\textbf{Object labels.}
We consider two object labels: an unsupervised binary saliency map called BigBiGAN \cite{voynov2021object} and a weakly-supervised multi-class prediction map called ReLabel \cite{yun2021re}. The object labelers are either trained on each downstream dataset or pretrained on ImageNet dataset \cite{deng2009imagenet}. Here, the two object labelers show comparable performance (see Table~\ref{tab:cls-more}); hence, we use the pretrained object labeler as default to reduce the cost of training a specific model for each dataset. Also, we use ReLabel if not specified since it performs better than BigBiGAN in most cases. We train a ResNet-18 \cite{he2016deep} network to obtain ReLabel on the downstream dataset, and use the publicly available BigBiGAN and ReLabel (NFNet-F6 \cite{brock2021high} version) trained on the ImageNet dataset for pretrained object labelers.

\textbf{Computation time.}
Training of the baseline DeiT-T on ImageNet takes 84 hours on 4 RTX 2080 Ti GPUs and 40 CPU cores (Intel Xeon Silver 4210R). ReMixer only increases the training and inference time slightly ($\times$1.1 longer).
